# Supplementary material for: Neighborhood Homophily-based Graph Convolutional Network
Source: arXiv:2301.09851 source file (2023-10-06)
Supplement: Supplementary file 1 [file appendix.tex]

% \appendix
\section{Dataset Details}\label{app:datasets}
For all datasets, we follow GPRGNN~\cite{chien2020adaptive} since it is well open-sourced. All datasets used in the ACM-GCN method~\cite{luan2022acm} differed in the number of edges from the same datasets used in the other methods, so we re-run the source code of the ACM-GCN method on the uniform datasets (used by GPRGNN). The results are post on Tab.~\ref{tab:main}. We also present the results from their paper in the Tab.~\ref{tab: app-result}.
Exploring minor differences in the datasets is not the focus of this paper.

\section{Baseline Details}\label{app:baselines}
\begin{itemize}
    \item \textbf{Two-layer MLP} is a neural network without propagation and aggregation rules and only learns node representations from node features.
    \item \textbf{GCN} is a graph convolutional network that aggregates information from the neighborhood on average.
    \item \textbf{GCNII} is a graph neural network using two effective tricks on the basis of GCN: initial residual and identity mapping.
    \item \textbf{BernNet} is a graph neural network that uses Bernstein polynomial approximation to design frequency filters.
    \item \textbf{GPRGNN} adaptively optimizes the Generalized PageRank weights to control the contribution of the propagation process at each layer.
    \item \textbf{ACM} adaptively mixes low-pass, high-pass, and identity channels node-wise before the GCN model to extract more information and address harmful heterophily. As for ACM+ (which uses layer normalization) and ACM++ (which uses residual), we believe that these general tricks do not reflect the ability of the model itself, and the original version of ACM and its variants (ACMII) also have high levels on various datasets, but for the sake of conciseness, we choose ACM as our baseline (the same reason for GCNII rather than GCNII*).
    \item \textbf{FAGCN} is a frequency adaptive graph neural network, which can adaptively aggregate low-frequency and high-frequency information.
    \item \textbf{GBK} uses homophilous and heterophilous weight matrices to obtain homophilous and heterophilous information, and then adaptively selects the appropriate weight matrix for the node pairs according to the gating mechanism. 
    \item \textbf{HOG} utilizes topology and attribute information of graphs to learn homophily degree between node pairs so that it can go beyond the homophily assumption (change the propagation rules under the homophily assumption).
%    \item \textbf{WRGAT} \red{runs GAT on a multi-relational graph containing both proximity and structural information.}
    \item\textbf{WRGAT} promotes assortativity node-wise of graph by building a multi-relational graph on top of the original graph to improve performance (The paper observes that higher assortativity leads to stronger predictive performance).
\end{itemize}

\section{Hyper-parameter Searching Space and Optimal Hyper-parameter Setting}\label{app:hyper}

\subsection{Common parameter Searching Space}
Table~\ref{tab: common-para} shows the searching space of several common parameters, including learning rate, weight decay, dropout and hidden dimension. We use a Tesla A100 40GB for model training and parameter tuning of all models, considering the modest size of the dataset.
\begin{table}[htp]
    
    \centering
    \caption{The searching space for the common parameters of all methods.}
    \resizebox{0.7\linewidth}{!}{
    \begin{tabular}{l|l} 
    \hline
    Parameter        & \multicolumn{1}{c}{Searching space}                                            \\ 
    \hline
    learning rate    & \multicolumn{1}{c}{\{0.001, 0.002, 0.005, 0.008, 0.01, 0.02, 0.05, 0.08, 0.1\}}  \\
    weight decay     & \{0, 5e-5, 1e-4, 5e-4, 1e-3, 5e-3\}                                             \\
    dropout          & \{0, 0.1, 0.2, 0.3, 0.4, 0.5, 0.6, 0.7, 0.8, 0.9\}                               \\
    hidden dimension & \{64, 128, 256, 512\}                                                          \\
    \hline
    \end{tabular}}
    \label{tab: common-para}
\end{table}

\subsection{Specific Parameters for Baselines}
We present some specific default parameters for several baseline models. 
For GPRGNN, we set the order of graph filter (frequency-domain filters often use finite orders) to 10 and the dropout rate before the propagation of GPR weights to 0.5, like BernNet, and let the coefficients $\gamma_k$ be initialized by PPR and set the $\alpha$ to 0.5. 
% 准确的表述参数名
For FAGCN, the residual coefficient $\epsilon$ of initial feature is set to 0.3. 
For WRGAT, the relations of multi-relational computation graph is set to 10. 
For HOG, all parameter settings follow the authors' settings. 
For GBK, the hyper-parameter $\lambda$ to balance two losses is set to 30. 
And other models follow the default public parameter settings.

\subsection{Parameter for NHGCN and NHGCN-SS}
Our method contains both common and specific parameters, shown in Table~\ref{tab: common-para} and Table~\ref{tab: specific-para}, respectively.
\textit{Activation function} will be chosen between ReLU and tanh, as~\cite{luan2019snowball} highlight the advantage of tanh in maintaining feature differentiation.
\textit{Hop} is chosen from $\{1, 2, 3\}$ because we consider the \textit{NH} of a node as a local metric, and different graphs have different applicability to locality assumption.
\textit{Add self-loop} refers to whether the self-loop is added in the GCN-like aggregation, i.e., \textit{Yes} means adopting 
$\operatorname{norm}(\boldsymbol{A})=(\boldsymbol{D}+\mathbf{I})^{-1/2}(\boldsymbol{A}+\boldsymbol{I})(\boldsymbol{D}+\boldsymbol{I})^{-1/2} $ 
and \textit{No} means adopting 
$\operatorname{norm}(\boldsymbol{A})=\boldsymbol{D}^{-1/2}\boldsymbol{A}\boldsymbol{D}^{-1/2} $. 
\textit{Combiner} will pick from three commonly used ones, including $\{add, concatenate, maxpooling\}$ , as described in Eq.~(\ref{eq: combinator}).
The threshold $T$ used to distinguish between high and low \textit{NH} groups is only adjusted as the denominator. For brevity, it is presented as an inverted form $1/T$ in Table~\ref{tab: specific-para}. 
$1/T$ practically varies from 2 to C, in 0.1 intervals, as well as two quartiles of .25 and .75. It starts from 2 because $1/T < 2$ means that one class is in the majority and the neighborhood label distribution has not yet reached the point where it can be measured using \textit{NH} metric.
% 强行解释
We use open source toolkit NNI~\cite{nni2021} and its built-in TPE~\cite{bergstra2011algorithms} algorithm to tune the hyper-parameters according to the validation accuracy. The optimal parameters are presented in Tab.~\ref{tab: para-nhgcn} and~\ref{tab: para-nhgcnss}.

\begin{table}[htp]

\centering
\caption{Specific Hyper-parameter Searching Space for NHGCN and NHGCN-SS.}
\resizebox{0.7\linewidth}{!}{
\begin{tabular}{l|l} 
\hline
Parameter           & \multicolumn{1}{c}{Searching space}                                      \\ 
\hline
activation function & \{ReLU, tanh\}                                                           \\
hop                & \{1, 2, 3\}                                                              \\
add self-loop            & \{Yes, No\}                                                              \\
combiner          & \{add, concatenate, maxpooling\}                                         \\
$1/T$         & \{2, 2.1, 2.2, 2.25, 2.3, 2.4, 2.5, 2.6, 2.7, 2.75, 2.8, 2.9, 3, $\cdots$, C\}  \\
\hline
\end{tabular}}
\label{tab: specific-para}
\end{table}

\begin{table*}[htp]

\centering
\caption{Optimal parameters for NHGCN}
\resizebox{\textwidth}{!}{
\begin{tabular}{c|ccccc|ccccc} 
\hline
                            & Cora & Citeseer & Pubmed & Photo & Computers & Chameleon & Actor & Squirrel & Texas & Cornell  \\ 
\hline
hidden dimension                & 512  & 512      & 512    & 512   & 512       & 512       & 512   & 512      & 512   & 64       \\
learning rate               & 0.1  & 0.001    & 0.1    & 0.05  & 0.05      & 0.002     & 0.1   & 0.002    & 0.08  & 0.01     \\
weight decay                & 1e-3 & 0        & 1e-4   & 5e-5  & 5e-5      & 0         & 1e-3  & 0        & 1e-4  & 5e-4     \\
dropout (aggregation layer) & 0.9  & 0.7      & 0.5    & 0.9   & 0.4       & 0         & 0.7   & 0.4      & 0.7   & 0.6      \\
dropout (combiner)        & 0.3  & 0.5      & 0      & 0.7   & 0.4       & 0.7       & 0.5   & 0.6      & 0.5   & 0.5      \\
activation function                 & ReLU & ReLU     & ReLU   & ReLU  & ReLU      & tanh      & ReLU  & tanh     & ReLU  & ReLU     \\
hop                        & 1    & 1        & 1      & 3     & 1         & 2         & 2     & 1        & 1     & 3        \\
add self-loop                    & Yes  & Yes      & Yes    & No    & No        & No        & Yes   & No       & No    & No       \\
combiner                  & maxpooling  & maxpooling      & add    & maxpooling   & add       & add       & add   & maxpooling      & add   & maxpooling      \\
$1/T$                   & 2.25 & 3.25     & 3.5    & 3.75  & 4         & 4.1       & 3.5  & 4        & 5     & 3.8   \\
\hline
\end{tabular}}
\label{tab: para-nhgcn}
\end{table*}

\begin{table*}[htp]

\centering
\caption{Optimal parameters for NHGCN-SS}
\resizebox{\linewidth}{!}{
\begin{tabular}{c|ccccc|ccccc} 
\hline
                            & Cora & Citeseer & Pubmed & Photo & Computers & Chameleon & Actor & Squirrel & Texas & Cornell  \\ 
\hline
hidden dimension                & 256  & 512      & 512    & 128   & 64        & 512       & 512   & 256      & 512   & 64       \\
learning rate               & 0.05 & 0.001    & 0.1    & 0.08  & 0.1       & 0.002     & 0.1   & 0.001    & 0.1   & 0.01     \\
weight decay                & 0    & 0        & 1e-4   & 5e-5  & 5e-5      & 0         & 1e-3  & 5e-5     & 1e-3  & 5e-4     \\
dropout (aggregation layer) & 0.9  & 0.6      & 0.5    & 0.8   & 0.6       & 0         & 0.8   & 0        & 0.5   & 0.4      \\
dropout (combiner)        & 0.4  & 0.3      & 0.6    & 0     & 0.3       & 0.6       & 0.9   & 0.5      & 0     & 0.5      \\
activation function                  & ReLU & ReLU     & ReLU   & ReLU  & ReLU      & tanh      & ReLU  & tanh     & ReLU  & ReLU     \\
hop                        & 3    & 3        & 2      & 1     & 3         & 1         & 1     & 1        & 3     & 1        \\
add self-loop                   & Yes    & Yes        & Yes      & No     & No         & No         & Yes     & No        & Yes     & No        \\
combiner                  & maxpooling  & maxpooling      & concatenate    & add   & add       & maxpooling       & concatenate   & add      & concatenate   & maxpooling      \\
$1/T$                  & 4    & 3.5      & 3      & 3     & 6         & 4.25      & 4.75  & 4.75     & 4.8   & 3.7     \\
\hline
\end{tabular}}
\label{tab: para-nhgcnss}
\end{table*}

% \newpage
\section{Full comparison}\label{app:full-compare}
We compare our results with those provided in the original papers of baselines except for FAGCN. Since no exact values are provided in its original paper, we adopt the experimental results of FAGCN from the ACM. These models in Table~\ref{tab: app-result} have achieved the current SOTA with dataset split of 60\% / 20\% / 20\% for training / validation / testing. 
The results of these models are relatively close on homophilous datasets and exhibit relatively larger gaps on heterophilous datasets.

\begin{table}[htp]
    
    \centering
    \caption{Results on real-world benchmark datasets reported in the original papers: 
    Mean Test Accuracy (\%) $\pm$ Standard Deviation (\%). Boldface letters are used to mark the best results while underlined letters indicate the second best.
    ``DS'' means that the dataset split is different from 60\% / 20\% / 20\%. 
    ``-'' means that the original paper has no experimental results on this dataset.}
    \resizebox{\linewidth}{!}{
    \begin{tabular}{c|ccccc|ccccc} 
    \hline
            & \textit{Cora} & \textit{Citeseer} & \textit{Pubmed} & \textit{Computers} & \textit{Photo} & \textit{Chameleon} & \textit{Actor} & \textit{Squirrel} & \textit{Texas} & \textit{Cornell}  \\ 
    \hline
    GeomGCN-I-g & 86.26         & 80.64             & 90.72           & -                  & -              & 68.00                 & 31.96          & 46.01             & 72.51          & 65.4              \\
    GBK     & 88.69 $\pm$ 0.42  & 79.18 $\pm$ 0.96      & 89.11 $\pm$ 0.23    & -                  & -              & -                  & 38.97 $\pm$ 0.97   & -                 & 81.08 $\pm$ 4.88   & 74.27 $\pm$ 2.18      \\
    GloGNN++   & 88.33 $\pm$ 1.09  & 77.22 $\pm$ 1.78      & 89.24 $\pm$ 0.39    & -                  & -              & \uline{71.21 $\pm$ 1.84}       & 37.70 $\pm$ 1.40   & \uline{57.88 $\pm$ 1.76}      & 84.05 $\pm$ 4.90   & 85.95 $\pm$ 5.10      \\
    GCNII*    & 88.01         & 77.13             & 90.3            & -                  & -              & 62.48              & -              & -                 & 77.84          & 76.49             \\
    GPRGNN     & 88.65 $\pm$ 0.28  & 80.01 $\pm$ 0.28      & 89.18 $\pm$ 0.15    & DS                  & DS              & 67.48 $\pm$ 0.40       & 39.30 $\pm$ 0.27   & 49.93 $\pm$ 0.53      & 92.92 $\pm$ 0.61   & 91.36 $\pm$ 0.70      \\
    CPGNN   & 83.76 $\pm$ 1.81  & 67.93 $\pm$ 2.86      & 82.44 $\pm$ 0.58    & -                  & -              & 67.19 $\pm$ 2.18       & -              & 54.76 $\pm$ 2.01      & 63.78 $\pm$ 7.67   & -                 \\
    ACMII-GCN+     & \textbf{89.18 $\pm$ 1.11}  & 81.87 $\pm$ 1.38      & 90.96 $\pm$ 0.62    & -                  & -              & \textbf{75.51 $\pm$ 1.58}       & 41.50 $\pm$ 1.54   & \textbf{69.81 $\pm$ 1.11}      & \textbf{95.41 $\pm$ 2.82}   & \textbf{93.93 $\pm$ 3.03}      \\
    BernNet & 88.52 $\pm$ 0.95  & 80.09 $\pm$ 0.79      & 88.48 $\pm$ 0.41    & 87.64 $\pm$ 0.44       & 93.63 $\pm$ 0.35   & 68.29 $\pm$ 1.58       & 41.79 $\pm$ 1.01   & 51.35 $\pm$ 0.73      & 93.12 $\pm$ 0.65   & \uline{92.13 $\pm$ 1.64}      \\
    FAGCN   & 88.85 $\pm$ 1.36            & \textbf{82.37 $\pm$ 1.46}                & 89.98 $\pm$ 0.54             & -                  & -              & 49.47 $\pm$ 2.84                 & 31.59 $\pm$ 1.37             & 42.24 $\pm$ 1.20               & 88.85 $\pm$ 4.39             & 88.03 $\pm$ 5.60                \\
    \hdashline
     NHGCN                                                & \uline{89.05 $\pm$ 1.00}          & 81.95 $\pm$ 0.85         & \uline{91.58 $\pm$ 0.54}  & \textbf{90.73 $\pm$ 0.55} & \textbf{95.24 $\pm$ 0.52}                                               & 69.85 $\pm$ 1.14 & \uline{42.86 $\pm$ 1.25}  & 51.02 $\pm$ 1.25          & 93.61 $\pm$ 3.32  & 90.64 $\pm$ 4.51                        \\
    NHGCN-SS                                             & 88.72 $\pm$ 1.61          & \uline{82.18 $\pm$ 0.97} & \textbf{91.64 $\pm$ 0.40} & \uline{90.72 $\pm$ 0.64}  & \uline{95.23 $\pm$ 0.41}                                             & 68.99 $\pm$ 1.63          & \textbf{42.94 $\pm$ 0.99} & 49.99 $\pm$ 1.74          & \uline{93.93 $\pm$ 2.19} & 91.28 $\pm$ 4.07  \\
    \hline
    \end{tabular}}
    \label{tab: app-result}
\end{table}
